# Supplementary material for: Multisection in the Stochastic Block Model using Semidefinite Programming
Source: arXiv:1507.02323 source file (2015-07-08)
Supplement: Supplementary file 1 [file Appendix.tex]

\subsection{Experimental Evaluation}
\label{sec:experiments}
In this section we present some experimental results on the SDPs presented
above. For both of the SDPs we consider the case of $p =
\alpha\frac{\log(m)}{m}$ and $q = \beta\frac{\log(m)}{m}$ with $k=3$ and $m =
20$. We vary $\alpha$ and $\beta$ and for each pair of values we take 10
independent instances and the shade of grey in the square represents the fraction of
instances for which the SDP was integral with lighter representing higher fractions of integrality. The red lines represent the curve we prove in our main
theorem \ref{thm:main_theorem_1_opt} i.e. $\sqrt{\alpha} - \sqrt{\beta} > 1$.

\begin{figure}[h!]
  \centering
    \includegraphics[width=0.7\textwidth]{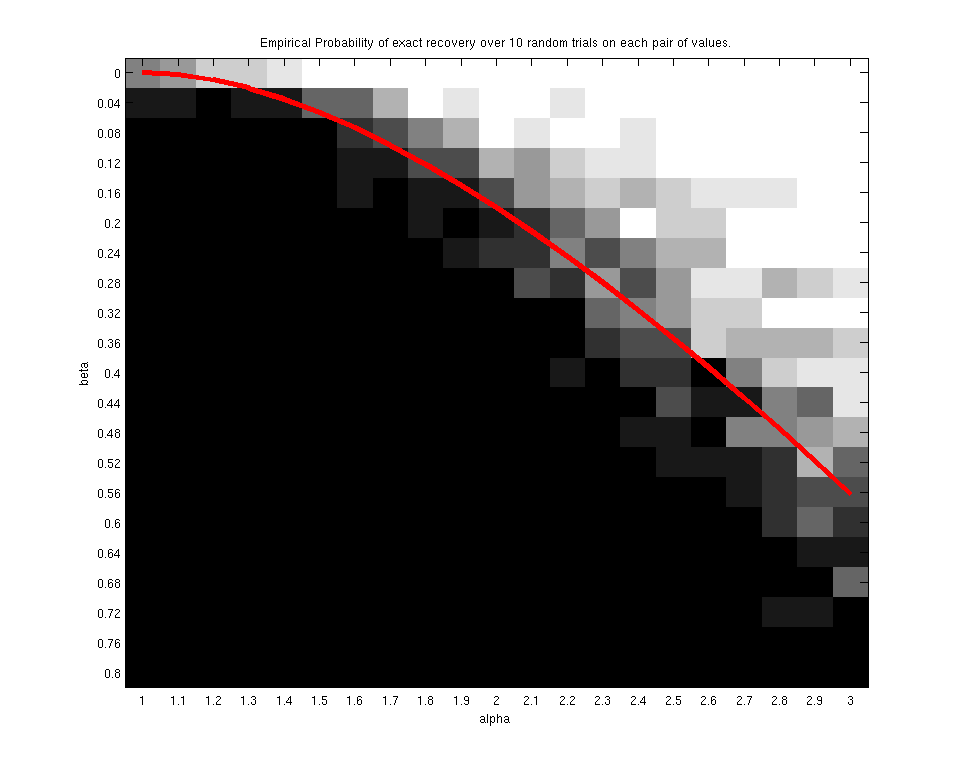}
    \caption{Performance of SDP in \eqref{eqn:sdp}. We consider the case of $p =
\alpha\frac{\log(m)}{m}$ and $q = \beta\frac{\log(m)}{m}$ with $k=3$ and $m =
20$. We vary $\alpha$ and $\beta$ and for each pair of values we take 10
independent instances and the shade of grey in the square represents the fraction of
instances for which the SDP was integral with lighter representing higher fractions of integrality. The red line represents the curve we prove in our main
theorem \ref{thm:main_theorem_1_opt} i.e. $\sqrt{\alpha} - \sqrt{\beta} > 1$.}
    \label{fig:sdp1}
\end{figure}

\begin{figure}[h!]
  \centering
    \includegraphics[width=0.7\textwidth]{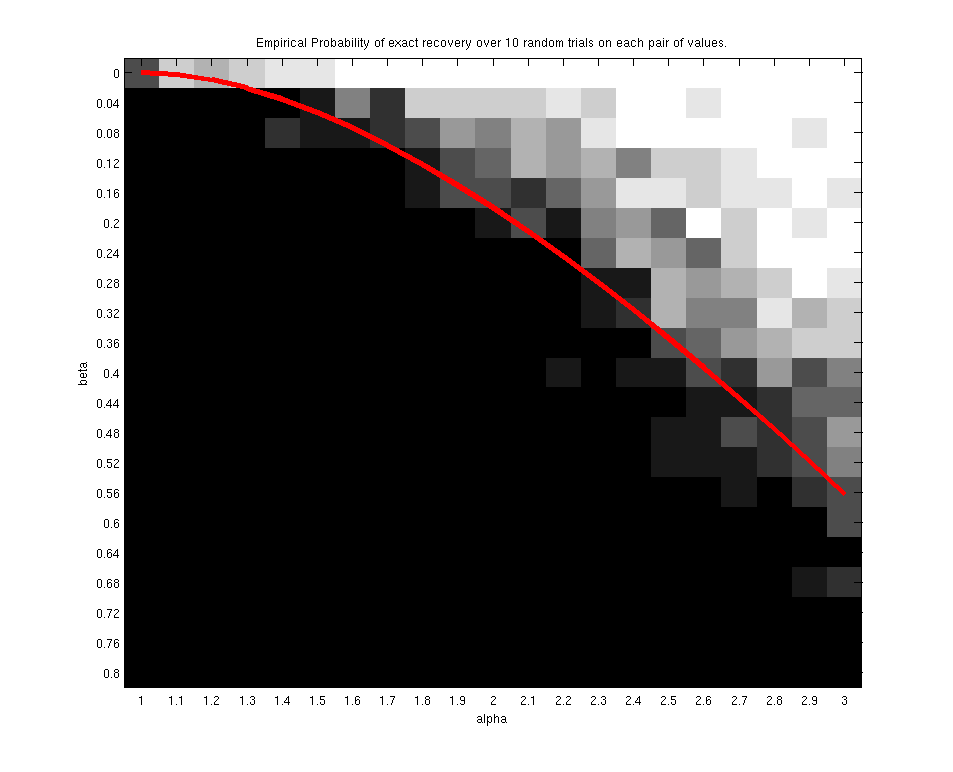}
	 \caption{Performance of SDP in \eqref{eqn:sdp2}. We consider the case of $p =
\alpha\frac{\log(m)}{m}$ and $q = \beta\frac{\log(m)}{m}$ with $k=3$ and $m =
20$. We vary $\alpha$ and $\beta$ and for each pair of values we take 10
independent instances and the shade of grey in the square represents the fraction of
instances for which the SDP was integral with lighter representing higher fractions of integrality. The red line represents the curve we prove in Theorem~\ref{thm:main_theorem_1_opt}, for the SDP~\eqref{eqn:sdp}, i.e. $\sqrt{\alpha} - \sqrt{\beta} > 1$.}
	\label{fig:sdp2}
\end{figure}

Figure \ref{fig:sdp1} corroborates our
theorem \ref{thm:main_theorem_1_opt} as for SDP in \eqref{eqn:sdp} we observe
that experimentally the performance almost exactly mimics what we prove. For the
other (possibly) weaker SDP in \eqref{eqn:sdp2} we see in Figure
\ref{fig:sdp2} that the performance is almost similar to the stronger SDP
however we were unable to prove it formally as discussed Section \ref{sec:sdps}. We leave this as an open question to show
that SDP in \ref{eqn:sdp2} is integral all the way down to the information theoretic threshold (i.e. $\sqrt{\alpha} - \sqrt{\beta} > 1$). We
observe from the experiments above that this indeed seems to be the case.

\subsection{The multireference alignment SDP for clustering}
\label{sec:nonuniquegames}
In this section we describe an interesting connection between the SDPs
used for clustering and partitioning problems and others such as ones used for
the multireference signal alignment and the unique games problems.
%Countless versions of the clustering problem exist. A particularly popular version of clustering a point cloud is $k$-means clustering~\cite{macqueen1967,Lloyd:kmeans}. On the graph side, there are extensions of the Cheeger's inequality (Theorem~\ref{CheegerInequality56}) to provide guarantees of spectral clustering in this setting~\cite{JRLee_SOGharan_LTrevisan_2011,SOGharan_LTrevisan_2011}. There are also adaptations of some of the ideas presented in Section~\ref{section:SBM2} to understand recovery in the Stochastic Block Model with multiple clusters~\cite{Agawarl_multisection_SBM,AbbeSandon15,Hajek_et_al_SBM_SDP_extensions}.

For illustrative purposes we will consider a slightly different version of the
balanced $k$-cut (multisection) problem described earlier. Instead of imposing
that the graph is partitioned in equal sized clusters, we will consider the objective value to be maximized to be
the difference between the number of \emph{agreeing pairs} and \emph{disagreeing pairs} where an
 agreeing pair is a pair of nodes connected by an edge that was picked to 
 be in the same cluster or a pair of points not connected by an edge that 
 is not in the same cluster, and disagreeing pairs are all the others. 
 Note that, if the balanced partition constraint was enforced, this objective would be equivalent to the multisection one.

The multireference alignment problem in signal processing~\cite{Bandeira_MRA} consists of aligning $n$ signals $y_1,\dots,y_n$ with length $k$ that are copies of a single signal but have been shifted and corrupted with white gaussian noise. For $a\in [k]$, we set $R_{l_i}$ to be the $k\times k$ matrix that shifts the entries of vector by $a$ coordinates. In this notation, the maximum likelihood estimator for the multireference alignment problem is given by the shifts $l_1,\dots,l_n\in [k]$ that maximize
\begin{equation}\label{eq:objectiformultireferenceappendix}
\sum_{i,j=1}^n \left\langle R_{l_i}^Ty_i, R_{l_j}^Ty_j \right\rangle = \sum_{i,j=1}^n \tr \left[ y_j y_i^T R_{l_i} R_{l_j}^T\right].
\end{equation}

A fruitful way of thinking about~\eqref{eq:objectiformultireferenceappendix} is as a sum, over 
each pair $i,j$, of pairwise costs that depends on the choices of shifts 
for the variable in each pair. An example of a problem of this type is the 
celebrated Unique Games problem, and indeed the SDP approach developed 
in~\cite{Bandeira_MRA} for the multireference alignment problem is an 
adaptation of an SDP based approximation algorithm for the Unique Games 
problems by Charikar et al.~\cite{CMM06}. The objective in the 
alignment problem~\eqref{eq:objectiformultireferenceappendix} has, 
however, an important property --- the pairwise costs only depends on the 
relative choices of shifts. More precisely, both $l_i$ and $l_j$ being 
increased by the same amount has no effect on the pairwise cost relative 
to $(i,j)$. In fact, there is a general framework for solving problems with 
this group invariance--type property, called non-unique games, when the 
group involved is compact~\cite{BCS15}. The example above 
and SDP~\eqref{eqn:sdp2} that we will derive below are particular cases of this framework, 
but it is more enlightening to derive the SDP we will use for partitioning 
from the multireference alignment one.

To obtain an SDP for the partitioning problem, one can think of each node $i$ as a 
signal $y_i$ in $\RR^k$ and think of a shift label as a cluster membership, the 
cost associated to the pair $i,j$ should then: if the nodes are connected, $+1$
if the two signals are given the same shift and $-1$ otherwise; if the nodes are
not connected it should be $-1$ if the two signals are given the same shift and
$+1$ otherwise. This can be achieved by replacing $y_jy_i^T$ on the objective~\eqref{eq:objectiformultireferenceappendix} by  appropriate $k\times k$ matrices $C_{ij}^T = \frac1{k}\left(2I - \1\1^T\right)$ if $i$ and $j$ are connected and $C_{ij}^T = \frac1{k}\left( \1\1^T - 2I\right)$ if not. Our objective would then be
\[
\sum_{a=1}^k\sum_{i,j\in \mathcal{C}_a}d_{ij} = - \sum_{i,j \in [n]} \tr \left[ C_{ij}^T R_{l_i}R_{l_j}^T  \right],
\]
where $R_{l_i}$ is constrained to be a circulant permutation matrix (a shift operator).

The SDP relaxation proposed in~\cite{Bandeira_MRA} would then take the form
 \begin{equation}\label{eq:def:generalSynchproblem:reprhoXX_MRA_SDP_cluster100}
\begin{array}{cl}
\max & \tr(CX) \\
\text{ s. t. } & X_{ii} = I_{k\times k} \\
 & X_{ij}\1 = \1\\
 & X_{ij} \text{ is circulant} \\
% & \left( X_{ij} \right)_{aa} = \left( X_{ij} \right)_{11}\\
% & \left( X_{ij} \right)_{ab} = \left( X_{ij} \right)_{12},\ \forall_{a\neq b}\\
 & X \geq 0 \\
 & X \succeq 0,
\end{array}
\end{equation}

It is clear, however, that~\eqref{eq:def:generalSynchproblem:reprhoXX_MRA_SDP_cluster100} has many optimal solutions. Given an optimal selection of cluster labelings, any permutation of these labels will yield a solution with the same objective. For that reason we can adapt the SDP to consider the average of such solutions. This is achieved by restricting each block $X_{ij}$ to be a linear combination of $I_{k\times k}$ and $\1\1^T$ (meaning that it is constant both on the diagonal and on the off-diagonal). Adding that constraint yields the following SDP.

 \begin{equation}\label{eq:def:generalSynchproblem:reprhoXX_MRA_SDP_cluster1}
\begin{array}{cl}
\max & \tr(CX) \\
\text{ s. t. } & X_{ii} = I_{k\times k} \\
 & X_{ij}\1 = \1\\
 & X_{ij} \text{ is circulant} \\
 & \left( X_{ij} \right)_{aa} = \left( X_{ij} \right)_{11}\\
 & \left( X_{ij} \right)_{ab} = \left( X_{ij} \right)_{12},\ \forall_{a\neq b}\\
 & X \geq 0 \\
 & X \succeq 0,
\end{array}
\end{equation}

Since the constraints in~\eqref{eq:def:generalSynchproblem:reprhoXX_MRA_SDP_cluster1} imply
\[
\left( X_{ij} \right)_{11} + (k-1) \left( X_{ij} \right)_{12} = 1,
\]
\eqref{eq:def:generalSynchproblem:reprhoXX_MRA_SDP_cluster1} can be described completely in terms of the variables $\left( X_{ij} \right)_{11}$. For that reason we consider the matrix $Z\in\RR^{n\times n}$ with entries $Z_{ij} = \left( X_{ij} \right)_{11}$. We can then rewrite~\eqref{eq:def:generalSynchproblem:reprhoXX_MRA_SDP_cluster1} as

 \begin{equation}\label{eq:def:generalSynchproblem:reprhoXX_MRA_SDP_cluster2}
\begin{array}{cl}
\max & \tr\left(\tilde{C}Z\right) \\
\text{ s. t. } & Z_{ii} = 1 \\
 & Z \geq 0 \\
 & Z^{(k)} \succeq 0,
\end{array}
\end{equation}
where $\tilde{C}_{ij} = kC_{ij}$ and $Z^{(k)}$ is the $nk\times nk$ matrix whose $n\times n$ diagonal blocks are equal to $Z$ and whose $n\times n$ non-diagonal blocks are equal to $\frac{11^T-Z}{k-1}$. For example,
\[Z^{(2)} = \left[\begin{array}{cc}
Z & 11^T-Z \\
 11^T-Z & Z 
\end{array}\right]
\quad\text{and}\quad Z^{(3)} = \left[\begin{array}{ccc}
Z & \frac{11^T-X}2 & \frac{11^T-Z}2 \\
\frac{11^T-Z}2 & Z & \frac{11^T-Z}2 \\
\frac{11^T-Z}2 & \frac{11^T-Z}2 & Z 
\end{array}\right].
\]

The following lemma gives a simpler characterization for the intriguing $Z^{(k)} \succeq 0$ constraint.

\begin{lemma}\label{eq_constraints_usesFourier}
 Let $Z$ be a symmetric matrix and $k\geq 2$ an integer.  $Z^{(k)} \succeq 0$ if and only if $Z \succeq \frac{1}k \1\1^T$.
\end{lemma}

Before proving Lemma~\ref{eq_constraints_usesFourier} we note that it implies that we can succinctly rewrite~\eqref{eq:def:generalSynchproblem:reprhoXX_MRA_SDP_cluster2} as
 \begin{equation}\label{eq:def:generalSynchproblem:reprhoXX_MRA_SDP_cluster3}
\begin{array}{cl}
\max & \tr\left(\tilde{C}Z\right) \\
\text{ s. t. } & Z_{ii} = 1 \\
 & Z \geq 0 \\
 & Z \succeq \frac{1}k \1\1^T.
\end{array}
\end{equation}
A simple change of variables $Y = \frac{k}{k-1}Z -\frac1{k-1}\1\1^T$, allows one to rewrite~\eqref{eq:def:generalSynchproblem:reprhoXX_MRA_SDP_cluster3} as (for appropriate matrix $C'$ and constant $c'$),
 \begin{equation}\label{eq:def:generalSynchproblem:reprhoXX_MRA_SDP_cluster_MaxKCut}
\begin{array}{cl}
\max & \tr\left(C'Y\right) - c' \\
\text{ s. t. } & Y_{ii} = 1 \\
 & Y_{ij} \geq -\frac1{k-1} \\
 & Y \succeq 0.
\end{array}
\end{equation}
Remarkably,\eqref{eq:def:generalSynchproblem:reprhoXX_MRA_SDP_cluster_MaxKCut} 
coincides with the classical semidefinite relaxation for the 
Max-k-Cut problem~\cite{FJ95}, 
which corresponds to~\eqref{eqn:sdp2} used in this paper.

\proof{[of Lemma~\ref{eq_constraints_usesFourier}]

Since, in this proof, we will be using $\1$ to refer to the all-ones vector in two different dimensions we will include a subscript denoting the dimension of the all-ones vector.

The matrix $Z^{(k)}$ is block circulant and so it can be block-diagonalizable by a block DFT matrix, $ F_{k\times k} \otimes I_{n\times n}$, where $F_{k\times k}$ is the $k\times k$ (normalized) DFT matrix and $\otimes$ is the Kronecker product. In other words,
\[
 \left(F_{k\times k}\otimes I_{n\times n}\right)Z^{(k)}\left( F_{k\times k}\otimes I_{n\times n}\right)^T
\]
is block diagonal. 
Furthermore, note that
\[
Z^{(k)} = \left(\1_k\1_k^T \otimes \frac{\1_n\1_n^T-Z}{k-\1}\right) - \left(I_{k\times k} \otimes  \left[ Z- \frac{\1_n\1_n^T-Z}{k-1}\right]\right).
\]
Also, It is easy to check that
\[
\left(F_{k\times k}\otimes I_{n\times n}\right)\left(I_{k\times k} \otimes \left[ Z- \frac{\1_n\1_n^T-Z}{k-1}\right]\right)\left(F_{k\times k}\otimes I_{n\times n}\right)^T = I_{k\times k} \otimes  \left[ Z- \frac{\1_n\1_n^T-Z}{k-1}\right],
\]
and
\[
\left(F_{k\times k}\otimes I_{n\times n}\right)\left(\1_k\1_k^T \otimes \frac{\1_n\1_n^T-Z}{k-1}\right)\left(F_{k\times k}\otimes I_{n\times n}\right)^T = k\left( e_1e_1^T \otimes \frac{\1_n\1_n^T-Z}{k-1}\right),
\]

This means that $ \left(F_{k\times k}\otimes I_{n\times n}\right)Z^{(k)}\left( F_{k\times k}\otimes I_{n\times n}\right)^T$ is a block diagonal matrix with the first block equal to $\mathcal{A}$ and all other diagonal blocks equal to $\mathcal{B}$ where $\mathcal{A}$ and $\mathcal{B}$ are given by
\[
\mathcal{A} = Z - \frac{\1_n\1_n^T-Z}{k-1} + k\frac{\1_n\1_n^T-Z}{k-1} =  \1_n\1_n^T \text{ and } \mathcal{B} =  Z- \frac{\1_n\1_n^T-Z}{k-1}.
\]
Thus, the condition $Z^{(k)}\succeq 0$ is equivalent to $Z- \frac{\1_n\1_n^T-Z}{k-1}\succeq 0$ which can be rewritten as,
\[
 Z - \frac{1}k\1_n\1_n^T \succeq 0.
\]
\hfill \qedhere

}

\subsection{Proof of Optimality - Theorem \ref{thm:main_theorem_1_lower_bound}}
\label{sec:proofmaintheoremlowerbound}
\begin{proof}
The theorem follows directly from the lower bound presented in \cite{ABH14}.
They showed that \cite[Theorem 1]{ABH14} when we sample $G \sim G_{p,q,2}$
with $p = \alpha'\frac{\log(n)}{n}$ and $q = \beta'\frac{\log(n)}{n}$, it is
information theoretically impossible to correctly recover the clusters with high
probability if 
\[ \sqrt{\alpha'} - \sqrt{\beta'} < \sqrt{2}\]
Now consider $G \sim G_{p,q,k}$ with $p = \alpha\frac{\log(m)}{m}$ and $q =
\beta\frac{\log(m)}{m}$. Suppose that the algorithm was given the
membership of vertices in all the clusters except two of them. A direct
application of the above theorem yields that it is information theoretically impossible
to correctly recover the two unrevealed clusters with high probability if
\[ \sqrt{2\frac{\log(m)}{\log(n)}}(\sqrt{\alpha} - \sqrt{\beta}) < \sqrt{2}\]
which is equivalent to 
\[ \sqrt{\alpha} - \sqrt{\beta} < \frac{\log(n)}{\log(m)} = 1 +
\frac{\log(k)}{\log(m)} = 1 + o_n(1)\]
which proves the bound.
\end{proof}

\subsection{Proof of Optimality - Theorem \ref{thm:main_theorem_1_opt}}
\label{sec:proofmaintheoremupperbound}
\begin{proof}
We will use the condition of theorem \ref{thm:main_theorem_1} and the following
lemma, to prove theorem \ref{thm:main_theorem_1_opt}. 

\begin{lemma}
\label{lemma:optimalityLemma}
Let $p=\frac{\alpha\log(m)}{m}$ and $q = \frac{\beta\log(m)}{m}$. Let
$k = \gamma\log(m)$ (where $\gamma = O(1)$). Now we have that as long as 
\begin{equation}
\label{eqn:optimalitylemma1}
\sqrt{\alpha} -
\sqrt{\beta} > \sqrt{1 + c_1\sqrt{\beta\gamma}\left(1 +
\log\left(\sqrt{\frac{\alpha}{\beta}}\right)\right)} \end{equation}then for
sufficiently large $n$ we have that with probability at least $1 -
n^{-\Omega(1)}$ $\forall{i,t}$ \[ \delta^{in}(i) - \delta_{i \rightarrow P_t} > c_2\left(\sqrt{\beta\gamma}\log(n) +
\sqrt{\alpha\log(n)}\right)
\] where $c_2 > 0$ be any fixed number and $c_1 > 0$ in
\eqref{eqn:optimalitylemma1} is a constant depending on $c_2$
\end{lemma}

To complete the proof of theorem \ref{thm:main_theorem_1_opt} we first observe
that for the given range of parameters $p = \frac{\alpha\log(m)}{m}$ and $q
= \frac{\beta\log(m)}{m}$ condition \eqref{eqn:condition} in Theorem
\ref{thm:main_theorem_1} becomes \[\hat{c}\left(\sqrt{pn/k + qn}
+ q\sqrt{\frac{n}{k}\log(n)} + \sqrt{\log(n)} + \log(k)\right) \leq 
c_2\left(\sqrt{\beta k\log(m)} + \sqrt{\alpha\log(n)}\right) 
\] However, Lemma \ref{lemma:optimalityLemma} implies that with probability $1 - n^{-\Omega(1)}$ we
have that if condition \ref{eqn:optimalitylemma1} is satisfied then $\forall{i,t}$ \[ \delta^{in}(i) - \delta_{i \rightarrow P_t} >
c_2\left(\sqrt{\beta\gamma}\log(n) + \sqrt{\alpha\log(n)}\right)
\]
where $c_2 > 0$ depends on $\hat{c}$. Therefore with probability $1 -
n^{-\Omega(1)}$ the condition in \eqref{eqn:condition} of Theorem \ref{thm:main_theorem_1} is satisfied which in
turn implies the SDP in Theorem \ref{thm:main_theorem_1} recovers the clusters,
which concludes the proof of Theorem \ref{thm:main_theorem_1_opt}. Note that
setting $\gamma = o(1)$ we get the case $k = o(\log(n))$ and the above condition
reduces to $\sqrt{\alpha} - \sqrt{\beta} > 1 + o_n(1)$.
\end{proof}

In the rest of the section we prove Lemma \ref{lemma:optimalityLemma}. For the
remainder of this section we borrow the notation from Abbe et al. \cite{ABH14}. In \cite[Definition 3, Section A.1]{ABH14}, they define the following quantity $T(m,p,q,\delta)$ which we use:
\begin{definition}Let $m$ be a natural number, $p, q \in [0, 1]$, and $\delta \geq 0$, define
$$T(m,p,q,\delta)=\prob \left[\sum_{i=1}^m(Z_i-W_i)\geq \delta \right] \:,$$
where $W_i$ are i.i.d Bernoulli$(p)$ and $Z_i$ are i.i.d. Bernoulli$(q)$, independent of the $W_i$.
\end{definition}

 Let $Z=\sum_{i=1}^mZ_i$ and $W=\sum_{i=1}^mW_i$. The proof is similar to proof of \cite[Lemma 8, Section A.1]{ABH14} with 
modifications.
\begin{proof}(of Lemma \ref{lemma:optimalityLemma})
We will bound the probability of the bad event
\[ \delta^{in}(i) - \delta_{i \rightarrow P_t} \leq
c_2\left(\sqrt{\beta\gamma}\log(n) +
\sqrt{\alpha\log(n)}\right) \:. \] 
Note that $\delta_{in}(i)$ is a binomial variable with parameter $p$ and
similarly $\delta_{i \rightarrow P_t}$ is a binomial variable with parameter
$q$ and therefore, following the notation of \cite{ABH14}, we have that the probability of this bad
event is \[T\left(m,p,q,-c_2\left(\sqrt{\beta\gamma}\log(n) +
\sqrt{\alpha\log(n)}\right)\right) \:.\]
We show the following strengthening of their lemma. 

\begin{lemma}
\label{lemma:appABH8}
Let $W_i$ be a sequence of i.i.d Bernoulli$\left(\frac{\alpha\log(m)}{m}\right)$
random variables and $Z_i$ an independent sequence of i.i.d
Bernoulli$\left(\frac{\beta\log(m)}{m}\right)$ random variables, then the
following bound holds for $m$ sufficiently large:
\begin{multline}
T\left(m,\frac{\alpha\log(m)}{m},\frac{\beta\log(m)}{m},
-c_2\left(\sqrt{\beta\gamma}\log(n) +
\sqrt{\alpha\log(n)}\right)\right) \leq \\
 \exp\left(
-\left( \alpha + \beta - 2\sqrt{\alpha\beta}
- c_1\sqrt{\beta\gamma}\left(1 +
\log\left(\sqrt{\frac{\alpha}{\beta}}\right) \right) + o(1) 
\right) \log(m) \right)
\end{multline}
where $c_2 > 0$ is a fixed number and $c_1 > 0$ depends only on $c_2$.  
\end{lemma}
Assuming the above lemma and taking a union bound over all clusters and
vertices we get the following sequence of equations which proves Theorem
\ref{lemma:optimalityLemma}
\begin{eqnarray*}
&&\prob\left((\exists\, i,t)\: \delta^{in}(i) - \delta_{i \rightarrow P_t} \leq
c_2\left(\sqrt{\beta\gamma}\log(n) +
\sqrt{\alpha\log(n)}\right)\right) \\ 
&& \leq mk^2 \exp\left(
-\left(\alpha + \beta - 2\sqrt{\alpha\beta}
- c_1\sqrt{\beta\gamma}\left(1 +
\log\left(\sqrt{\frac{\alpha}{\beta}}\right) \right) + o(1) 
\right)\log(m) \right)\\
&& \leq \exp\left(
-\left(\alpha + \beta - 2\sqrt{\alpha\beta}
- 1 - c_1\sqrt{\beta\gamma}\left(1 +
\log\left(\sqrt{\frac{\alpha}{\beta}}\right) \right) + o(1) 
\right)\log(m) \right)\\
&& \leq m^{-\Omega(1)} \\
&& \leq n^{-\Omega(1)} 
\end{eqnarray*}
\end{proof}
\begin{proof}[Proof of Lemma \ref{lemma:appABH8}]
The proof of lemma \ref{lemma:appABH8} is a simple modification of the
proof of \cite[Lemma 8, Section A.1]{ABH14}. We mention the proof here
for completeness. 

Define $r = c_2\left(\sqrt{\beta\gamma}\log(n) +
\sqrt{\alpha\log(n)}\right) \leq c_1\sqrt{\beta\gamma}\log(n)$ (for
some fixed $c_1 > 0$ depending only on $c_2$) and let $Z = \sum Z_i$ and $W =
\sum W_i$.
We split $T$ as follows: \[ T(m,p,q,-r) = \prob\left( -r \leq Z-W \leq
\log^2(m)\right) + \prob\left(Z-W \geq \log^2(m)\right) \:. \] Lets bound
the second term first. A simple application of Bernstein's Inequality (the
calculations are shown in \cite[Lemma 8, Section A.1]{ABH14}) shows that 
Therefore we have that 
\[\prob\left(Z - W \geq \log^2(m)\right) \leq
\exp\left(-\Omega(1)\frac{\log^2(m)}{\log(\log(m))}\right) \:.\]
We now bound the first term $\prob\left( -r \leq Z-W \leq
\log^2(m)\right)$. Define 
\[ \hat{r} = argmax_{x} \prob(Z-W = -x) \]
Now it is easy to see that $\hat{r} = O(\log(m))$ (for
$p=\alpha\frac{\log(m)}{m}$ and $q = \beta\frac{\log(m)}{m}$).
Let $r_{max} = \max(r,\hat{r})$ and $r_{min} = \min(r,\hat{r})$. 

\begin{align*}
\prob\left(-r \leq Z - W\leq \log^2(m)\right)   &\leq (\log^2(m)
+ r_{max})\prob(Z - W = -r_{min}) \\[1em]
&\leq \begin{aligned}
(\log^2(m) + r_{max})\left(\sum_{k_2=r_{min}}^{\log^2(m)+r_{max}} \prob(Z=k_2 -
r)\prob(W=k_2)  \right. \\ 
+ \left. \sum_{k_2 = \log^2(m)+r_{min}}^m \prob(Z=k_2 -
r)\prob(W=k_2)\right) 
\end{aligned}
\\[1em]
&\leq \begin{aligned}
(\log^2(m)+r_{max})^2 \max_{k_2}\{\prob(Z=k_2 -
r_{min})\prob(W=k_2)\} \\ + (\log^2(m)+r_{max})\prob(Z\geq \log^2(n))\prob(W\geq
\log^2(m))
\end{aligned}
\end{align*}
The first inequality follows easily from considering both the cases $\hat{r}
\geq r$ or $\hat{r} \leq r$.
Similar probability estimates (using Bernstein) as before give that both 
\[ \prob\left(Z\geq \log^2(m)\right), \prob\left(W\geq \log^2(m)\right) \leq 
\exp\left(-\Omega(1)\frac{\log(m)}{\log(\log(m))}\right)\]
We now need to bound $\max_{k_2}\{\prob(Z=k_2 - r)\prob(W=k_2)\}$ for which we use
Lemma \ref{lemma:appABH7} which is a modification of \cite[Lemma 7, Section A.1]{ABH14}. 
Plugging the estimates from above and noting that $\max_{k_2}\{\prob(Z=k_2 -
r)\prob(W=k_2)\} = T^*\left(m,p,q,\frac{r_{min}}{\log(m)}\right)$ (defined in
Lemma \ref{lemma:appABH7}) we get that
\begin{equation*}
\prob\left( -r \leq Z-W \leq
\log^2(m)\right) \leq O(\log^4(n))T^*\left(m,p,q,\frac{r_{min}}{\log(m)}\right)
+ \log^2(n)\exp\left(-\Omega(1)\frac{\log(m)}{\log(\log(m))}\right)
\end{equation*}
Putting everything together we get that
\begin{equation*}
T(m,p,q,0) \leq 2\log^4(n)T^*\left(m,p,q,\frac{r_{min}}{\log(m)}\right) +
\log^2(n)\exp\left(-\Omega(1)\frac{\log(m)}{\log(\log(m))}\right) +
\exp\left(-\Omega(1)\frac{\log(m)}{\log(\log(m))}\right)
\end{equation*}
Using Lemma \ref{lemma:appABH7} it follows from the above equation that 
\begin{eqnarray*}
-\log(T(m,p,q,-r)) &\geq& -\Omega(\log(\log(m)))
+ g\left(\alpha,\beta,\frac{r_{min}}{\log(n)} \right)\log(m) - o(\log(m))
\\
&\geq& \left(\alpha + \beta - 2\sqrt{\alpha\beta}
- c_1\sqrt{\beta}\gamma\left(1 +
\log\left(\sqrt{\frac{\alpha}{\beta}}\right) \right)\right)\log(m) - o(\log(m))
\end{eqnarray*}
For the first inequality we use Lemma \ref{lemma:appABH7} and set
$\epsilon = \frac{r_{min}}{\log(n)}$. For the second inequality we use the fact
that $\epsilon \leq c_1\sqrt{\beta\gamma}$.
\end{proof}
\begin{lemma}
\label{lemma:appABH7}
Let $p = \frac{\alpha\log(m)}{m}$ and $q = \frac{\beta\log(m)}{m}$ and let $W_i$
be a sequence of i.i.d Bernoulli-$p$ random variables and $Z_i$ an independent
sequence of i.i.d Bernoulli-$q$ random variables. Define
\begin{eqnarray*}
& & V'(m,p,q,\tau,\epsilon) = \prob\left(\sum Z_i =
\tau\log(m)\right)\prob\left(\sum W_i = (\tau+\epsilon)\log(m)\right)\\
& & = \binom{m}{\tau\log(m)}q^{\tau\log(m)}(1-q)^{m -
\tau\log(m)}\binom{m}{(\tau + \epsilon)\log(m)}p^{(\tau
+ \epsilon)\log(m)}(1 - p)^{m -
(\tau + \epsilon)\log(m)} \:,
\end{eqnarray*}
where $\epsilon = O(1)$. We also define the function
\[g(\alpha,\beta,\epsilon) = (\alpha + \beta) - \epsilon\log(\alpha) -
2\sqrt{\left(\frac{\epsilon}{2}\right)^2 + \alpha\beta} +
\frac{\epsilon}{2}\log\left(\alpha\beta \frac{\sqrt{(\frac{\epsilon}{2})^2 +
\alpha\beta} + \frac{\epsilon}{2}}{\sqrt{(\frac{\epsilon}{2})^2 + \alpha\beta} - \frac{\epsilon}{2}}\right) \:. \]
Then we have the following results for $T^*(m,p,q,\epsilon) = \max_{\tau >
0}V'(m,p,q,\tau,\epsilon)$ :
for $m \in N$ and $\forall \tau > 0$
\[ -\log(T^*(m,p,q,\epsilon)) \geq \log(m) g(\alpha,\beta,\epsilon) -
o\left(\log(m)\right) \:. \]
\end{lemma}

\begin{proof}
The proof of the above lemma is computational and follows from the carefully
bounding the combinatorial coefficients. Note that 
\begin{eqnarray*}
\log(V(m,p,q,\tau,\epsilon)) =&& \log\binom{m}{\tau\log(m)} +
\log\binom{m}{(\tau + \epsilon)\log(m)} + \tau\log(m)\log(pq) + \\&&
\epsilon\log(m)\log\left(\frac{p}{1-p} + (m - \tau\log(m))\log((1-p)(1-q))
\right)
\end{eqnarray*}
Substituting the values of $p$ and $q$ we get 
\begin{eqnarray*}
\log(V(m,p,q,\tau,\epsilon)) =&& \log\binom{m}{\tau\log(m)} +
\log\binom{m}{(\tau + \epsilon)\log(m)} \\&& + 
\tau\log(m)\left(\log(\alpha\beta) + 2\log\log(m) - 2\log(m)\right) \\&& + 
\epsilon\log(m)\left(\log(\alpha) + \log\log(m) - \log(m) +
\alpha\frac{\log(m)}{m} \right) \\&& - \log(m)(\alpha + \beta) + 
o(\log(m))
\end{eqnarray*} 
We now use the following easy inequality
\[ \log\binom{n}{k} \leq k\left( \log(ne) - \log(k) \right)\]
and now replacing this in the above equation gives us 
\begin{multline}
 -\log(V(m,p,q,\tau,\epsilon)) \geq \log(m)\left((\alpha + \beta) + (\tau
+ \epsilon)\log\left(\frac{\tau + \epsilon}{e}\right) +
\tau\log\left(\frac{\tau}{\epsilon}\right) - \tau\log(\alpha\beta) -
\epsilon\log(\alpha)\right) \\  - o(\log(m))
\end{multline}

Now optimizing over $\tau$ proves the lemma. 
\end{proof}
% 

% \begin{lemma}
% \label{lemma:optimalitylemma1}
% If $k$ is fixed then as long as
% $\frac{(p-q)n}{k\log(n)}$ is a constant greater than 1 then with probability $1
% - o(1)$ we can recover the clusters.
% \end{lemma}
% \begin{proof}
% Using lemma \ref{lemma:optimalitylemma2} we have that with probability $1 -
% o(1)$ we have that
% \[\min_i\{\delta_{in}(i) - \delta_{\max}^{out}(i)\} \geq
% \frac{(p-q)n}{k\log(\log(n))} \:.\]
% 
% \end{proof}
% 
% \begin{lemma}
% \label{lemma:optimalitylemma2}
% If $k$ is a constant (or may be a slow growing function of $n$) then as long as
% $\frac{(p-q)n}{k\log(n)}$ is a constant greater than 1 then with probability $1
% - o(1)$ we have that
% \[ \min_i\{\delta_{in}(i) - \delta_{\max}^{out}(i)\} \geq
% \frac{(p-q)n}{k\log(\log(n))} \:.\]
% For any i consider the quantity using the Chernoff bound mentioned in Theorem
% \ref{thm:chernoff} we get that
% 
% 
% \end{lemma}
% 
% \begin{theorem}
% For constant $k$, as long as 
% \[ \sqrt{\alpha} - \sqrt{\beta} > \sqrt{k} \]
% we can recover the clusters with probability $1 - o(1)$.
% \end{theorem}
% \begin{proof}
% Note that $\sqrt{\alpha} - \sqrt{\beta} \geq \sqrt{k} \Rightarrow \alpha -
% \beta \geq k$. Now consider $\frac{(p-q)n}{\log(n)} = \frac{\alpha -
% \beta}{k}$ which implies $\frac{(p-q)n}{\log(n)}$ is a constant greater than 1
% and the theorem now follows from Lemma \ref{lemma:optimalitylemma1}.
% \end{proof}

\subsection{Proofs of Lemmas for the SDP in \eqref{eqn:sdp}}
\subsection{Proof of lemma \ref{lem:main_lemma}}
\label{sec:proof_main_lemma}
We remind the reader that the proof of the lemma below continues the use of the
notation used in Section  \ref{sec:proof_main_theorem}
\begin{proof}
To prove this lemma we first show that Equation \ref{eqn:sumcondition} is
satisfied for $M^*$. This implies that the vectors $\{v_t\}$ which are indicator
vectors for the clusters are an eigenvector with eigenvalue 0. Consider the
value of $\delta_{i \rightarrow P_t}(M^*)$ when $P_t = P(i)$. In this case
\begin{eqnarray*}
\delta_{i \rightarrow P_t}(M^*) &=& D^*[i,i] + \frac{n}{k}x^*_i+
\sum_{i' \in P(i)}x^*_{i'} - \sum_{i' \in P(i)} A[i,i'] \\
&=& 0 \:. \\ 
\end{eqnarray*}
where the last equality follows directly from the definitions of the dual
certificate. Now consider the value of $\delta_{i \rightarrow P_t}(M^*)$ when
$P_t \neq P(i)$. In this case
% \begin{eqnarray*}
% &&\delta_{i \rightarrow P_t}(M^*) = n/k(x^*_i) +
% \sum_{j \in P_t}x^*_{i'} - \sum_{j \in P_t} Z[i,j] + A[i,j] \\
% &&= n/k(x^*_i) +
% \sum_{j \in P_t}x^*_{i'} - \left( \sum_{j \in P_t} 
% \frac{\delta^{out}_{\max}(i)}{n/k} + \frac{\delta^{out}_{\max}(j)}{n/k} -
% \left(\frac{\delta_{i \rightarrow P(j)}}{n/k} + A[i,j]\right)+ \left(  -
% \frac{\delta_{j \rightarrow P(i)}}{n/k} + \frac{\delta_{P(j) \rightarrow
% P(i)}}{(n/k)(n/k)}\right)  -
%                \min_{t_1,t_2} \frac{\delta_{P_{t_1} \rightarrow
%                P_{t_2}}}{(n/k)(n/k)} \right)\\
% &&= n/k(x^*_i) +
% \sum_{j \in P_t}x^*_{i'} - \left(\sum_{j \in P_t} 
% \frac{\delta^{out}_{\max}(i)}{n/k} + \frac{\delta^{out}_{\max}(j)}{n/k} -
%                \min_{t_1,t_2} \frac{\delta_{P_{t_1} \rightarrow
%                P_{t_2}}}{(n/k)(n/k)} \right) \\             
% &&= 0 \\ 
% \end{eqnarray*}

\begin{align*}
  \delta_{i \rightarrow P_t}(M^*) &= \begin{aligned}[t]
      &\frac{n}{k}x^*_i +
\sum_{j \in P_t}x^*_{j} - \sum_{j \in P_t} (Z[i,j] + A[i,j])
       \end{aligned}\\
   &= \begin{aligned}[t]
      &\frac{n}{k}x^*_i+
\sum_{j \in P_t}x^*_{j} - \sum_{j \in P_t} \left( 
\frac{\delta^{out}_{\max}(i)}{n/k} + \frac{\delta^{out}_{\max}(j)}{n/k} -
\left(\frac{\delta_{i \rightarrow P(j)}}{n/k} + A[i,j]\right)+\right.\\
      &\left. \left( -\frac{\delta_{j \rightarrow P(i)}}{n/k} +
      \frac{\delta_{P(j) \rightarrow P(i)}}{(n/k)(n/k)}\right)  - \min_{t_1,t_2} \frac{\delta_{P_{t_1} \rightarrow P_{t_2}}}{(n/k)(n/k)} \right )
       \end{aligned} \\
    &= \frac{n}{k}x^*_i + \sum_{j \in P_t}x^*_{j} - \sum_{j \in P_t} \left(
\frac{\delta^{out}_{\max}(i)}{n/k} + \frac{\delta^{out}_{\max}(j)}{n/k} -
               \min_{t_1,t_2} \frac{\delta_{P_{t_1} \rightarrow
               P_{t_2}}}{(n/k)(n/k)} \right) \\  
               &=0 \:.
\end{align*}
The third equality follows by noting that the terms in the parenthesis in the
expression in the second line go to zero in summation. The fourth equality
follows directly from the definitions.

The above implies that for all $t$, $M^*v_t = 0$. Therefore we only need to
show that $M^*$ is PSD with high probability on the subspace $\R_{n | k}$ (which is perpendicular to $\R_{k} = span(\{v_k\})$). To that end, note that if a
matrix $W$ is such that for all $i$, $W[i,j_1] = W[i,j_2]$ when $P(j_1) =
P(j_2)$ then for any $x \in \R_{n | k}, Wx = 0$, and similarly if for all $j$,
$W[i_1,j] = W[i_2,j]$ when $P(i_1) = P(i_2)$ then for any $x \in \R_{n | k},
x^TW = 0$. Therefore we have that $x^TZ^*x = x^T(R_i + C_i)x = 0$ and so
$x^TM^*x = x^TD^*x - x^TAx$. 

In order to finish the proof it is enough to show that for all $x
\in \R_{n | k}$
\begin{equation*} 
x^T(D^* - A)x \geq 0 \:.
\end{equation*}
In order to prove the above equation, and conclude the proof of Theorem
\ref{thm:main_theorem_1_restate} we use the following two lemmas, which we prove in the Appendix.

\begin{lemma}
\label{lemma:conc}
Define $\lambda_{max}(A(G))$ to be the maximum over all $x \in \R_{n | k}$ of
$x^TA(G)x$. With probability $1 - n^{-\Omega(1)}$ over the choice of $G$,
$\lambda_{max}(A(G))$ is bounded by \begin{equation} \label{eqn:conc} \lambda_{\max}(A(G)) \leq 3\sqrt{pn/k + qn} +
c\sqrt{\log(n)} \:. \end{equation}
where $c$ is a universal constant.
\end{lemma}
% We will also need the following estimate of $\Delta \defeq E[\delta^{in}(i) -
% \delta^{out}_{max}(i)]$
% \begin{lemma}
% \label{lemma:edelta}
% \begin{equation}
% \Delta \geq \frac{pn}{k} - \frac{qn}{k} - c'(\sqrt{\frac{qn}{k}\log(k)})
% \end{equation}
% for some universal constant $c'$
% \end{lemma}
\begin{lemma}
\label{lemma:deviationdiag}
With probability $1 - n^{-\Omega(1)}$ we have that for all clusters $P_t$
\begin{equation} \label{eqn:deviationdiag1} \sum_{j \in P_t}
\frac{\delta^{out}_{\max}(j)}{n/k} \leq \frac{qn}{k} +
30\left(\sqrt{\frac{n\log(k)}{k}q} + \log(k) + \sqrt{\frac{n}{k}\log(n)}\cdot
\max\left\{q,\sqrt{\frac{q\log(n)}{n/k}},\frac{\log(n)}{n/k}\right\}\right)\:,
\end{equation}
and for all pairs of clusters $P_{t_1}$ and $P_{t_2}$ 
\begin{equation} \label{eqn:deviationdiag2} \min_{t_1,t_2}
\frac{\delta_{P_{t_1} \rightarrow P_{t_2}}}{n/k} \geq \frac{qn}{k} -
2\sqrt{q\log(n)} \:.
\end{equation}
\end{lemma}

Using those two lemmas, we can now conclude the proof of Theorem
\ref{thm:main_theorem_1_restate} as follows:\\
We separate $D^* = D_1^* - D_2^*$, where $D_1^*,D_2^*$ are diagonal matrices
\begin{eqnarray*}
&& D_1^*[i,i] = \delta^{in}(i) - \delta^{out}_{\max}(i) \\
&& D_2^*[i,i] = \sum_{j \in P(i)} \frac{\delta^{out}_{\max}(j)}{n/k} -
\min_{t_1,t_2} \frac{\delta_{P_{t_1} \rightarrow P_{t_2}}}{n/k} \:.
\end{eqnarray*}
Now for any $x \in \R_{n | k}$ lets consider $x^T(D^* - A)x$
\begin{align*} 
x^T(D^* - A)x &\geq \min_i D_1^*[i,i] - \left(\max_{i}D_2^*[i,i] + \max_{x
\in \R_{n|k}}x^TAx\right) \\
&\begin{aligned} \geq
& \min_iD_1^*[i,i] - \left( 30\left(\sqrt{\frac{n\log(k)}{k}q} + \log(k) +
\sqrt{\frac{n}{k}\log(n)}\cdot
\max\left\{q,\sqrt{\frac{q\log(n)}{n/k}},\frac{\log(n)}{n/k}\right\}\right) 
\right.
\\
& \left.+ 3\sqrt{pn/k + qn}
+ c\sqrt{\log(n)}\right)
\end{aligned}  \\
&\geq \min_iD_1^*[i,i] - \hat{c}\left(\sqrt{pn/k + qn} +
q\sqrt{\frac{n}{k}\log(n)} + \sqrt{\log(n)} + \log(k)\right) \\
&\geq 0 \:.
\end{align*}
where $\hat{c}$ is a universal constant. The second inequality follows by direct
substitutions from Equations \ref{eqn:conc}, \ref{eqn:deviationdiag1}, \ref{eqn:deviationdiag2}, the third
inequlity follows from noting that $n$ is large enough such that $\sqrt{qn} >>
\sqrt{q}\log(n)$ and $\sqrt{\log(n)}\frac{\log(n)}{\sqrt{\frac{n}{k}}} <<
\sqrt{log(n)}$ and $\sqrt{qn\frac{\log(k)}{k}} \leq \sqrt{qn}$. The
last inequality follows from condition \ref{eqn:condition} of Theorem
\ref{thm:main_theorem_1_restate}.
\end{proof}

\subsubsection{Proof of Lemma \ref{lemma:conc}}
We use the following recent sharp concentration result \cite[Corollary~3.12]{BH14}.
\begin{theorem}[Bandeira et al. \cite{BH14}]
\label{thm:bh14}
Let X be an $n \times n$ symmetric matrix whose entries $X_{ij}$ are independent
centered random variables. Then there exists for any $0 < \epsilon \leq 1/2$ a
universal constant $\tilde{c_{\epsilon}}$ such that for every $t \geq 0$
\begin{equation*}
\prob\left( |X| \geq (1+\epsilon)2\sqrt{2}\tilde{\sigma} + t\right) \leq
ne^{-t^2/\tilde{c_{\epsilon}}\sigma^2_*} \:,
\end{equation*}
where 
\begin{equation*}
\tilde{\sigma} = \max_i \sqrt{\sum_j \expect[X_{ij}^2]}, \;\;\;\;\; \sigma_* =
\max_{ij}\|X_{ij}\|_{\infty} \:.
\end{equation*}
\end{theorem}
We apply the above theorem to the matrix $A - \expect[A]$. It is easy to see that the
variance of any row $\tilde{\sigma}$ is upper bounded by 
\[ \tilde{\sigma} \leq \sqrt{p(1-p)n/k + q(1-q)n} \leq \sqrt{pn/k +
qn}\:, \] and $\sigma_* \leq 1$. Applying theorem \ref{thm:bh14} with the
above parameters $\tilde{\sigma} = \sqrt{pn/k +
qn}$ and $\sigma_* = 1$, we get that with probability $1 - n^{-\Omega(1)}$ \[ |A -
\expect[A]| \leq 3\sqrt{pn/k + qn} + c'\sqrt{\log(n)} \:.\] where $c'$ is a
universal constant defined as $c' = 2\tilde{c_{\epsilon}}$ for $\epsilon =
\frac{3}{2\sqrt{2}} - 1$ and $\tilde{c_{\epsilon}}$ defined by the statement
of Theorem \ref{thm:bh14}. Also note that $\expect[A] + pI$ has the space
$\R_{n|k}$ as an eigenspace with eigenvalue 0. Therefore we have that for any
unit vector $x \in \R_{n|k}$ \begin{eqnarray*} |x^TAx| &\leq& |A - \expect[A]| +
|x^T \expect[A]x| \\
&\leq& 3\sqrt{pn/k +
qn} + c'\sqrt{\log(n)} + p \\
&\leq& 3\sqrt{pn/k + qn} + c\sqrt{\log(n)}\:.
\end{eqnarray*}
where $c = c' + 1$. This proves Lemma \ref{lemma:conc} 
\subsubsection{Proof of Lemma \ref{lemma:deviationdiag}}
\begin{proof}
We prove Lemma \ref{lemma:deviationdiag} using the following, which we prove in subsection \ref{subsec:edelta}.
\begin{lemma}
 \label{lemma:edelta}
 For every vertex $i$ we have that
 \begin{equation*}
 \expect\left[\delta^{out}_{\max}(i)\right] \leq 
 \frac{qn}{k} +
28\left(\sqrt{\frac{n\log(k)}{k}q} + \log(k)\right) \:.
 \end{equation*}
\end{lemma}

Using this, the proof of lemma \ref{lemma:deviationdiag} is as follows.
Note that by a direct application of the Chernoff bound described in Corollary
\ref{corr:mychernoffgood} and with a union bound over all clusters and
vertices we get that with probability $1 - \frac{1}{n}$ for all vertices $i$ and all
clusters $P_t \neq P(i)$ \[ \delta_{i \rightarrow P_t} \leq \frac{qn}{k} +
12\sqrt{\frac{qn}{k}\log(n)}+ 12\log(n) \:.\] 
Lets call the above event $\mathcal{E}$ and 
consider the sum \[S(i) = \frac{\sum_{i' \in P(i)} \delta_{\max}^{out}(i)}{n/k}
\:.\] Let
\[ \gamma = \frac{qn}{k} +
30\left(\sqrt{\frac{n\log(k)}{k}q} + \log(k) +
\sqrt{\frac{n}{k}\log(n)}\cdot
\max\left\{q,\sqrt{\frac{q\log(n)}{n/k}},\frac{\log(n)}{n/k}\right\}\right) \:.\]
We have that
\begin{eqnarray*}
\prob\left(\exists
i\:S(i) \geq  \gamma \right)  &=&
\prob(\mathcal{E})\prob\left(\exists
i\:S(i) \geq  \gamma \,|\,
\mathcal{E}\right) + \prob(\sim\mathcal{E})\prob\left(\exists
i\:S(i) \geq \gamma \,|\,
\sim\mathcal{E}\right)
\\
&\leq& n^{-\Omega(1)} + \prob\left(\exists
i\:S(i) \geq \gamma \,|\, \sim\mathcal{E}\right) \:.
\end{eqnarray*} 
Now for a fixed $i$ we will consider $\prob\left(S(i) \geq \gamma \,|\, \sim\mathcal{E}\right)$. Note that under the conditioning the
individual entries in the sum above are still independent, and therefore the above is an average of independent random
variables each of which is bounded by $\frac{qn}{k} +
12\sqrt{\frac{qn}{k}\log(n)}+ 12\log(n)$ (by the
conditioning). Also note that for any positive random variable $X$
\[\expect[X \,|\, \sim\mathcal{E}] \leq
\frac{\expect[X]}{\prob(\sim\mathcal{E})}\:,\] and since we have that
$\prob(\sim\mathcal{E}) \geq 1 - 1/n$, we get that \[\expect[S(i) \,|\,
\sim\mathcal{E}] \leq \expect[S(i)] + \frac{\expect[S(i)]}{n-1} \:.\] We
now use Hoeffding's inequality \ref{thm:Hoeffding} in the conditioned
probability space (and remove the conditioning terms from the
probability for ease of notation) to
get that \[ \prob(S(i) \geq \expect[S(i)] + t) \leq \exp\left(-\frac{2\frac{n^2}{k^2}t^2}{\frac{n}{k}\left(\frac{qn}{k} + 12\sqrt{\frac{qn}{k}\log(n)}+ 12\log(n)\right)^2}\right) \:.\] Now, if we choose 
\[t = 25\sqrt{\frac{n}{k}\log(n)}\cdot
\max\left\{q,\sqrt{\frac{q\log(n)}{n/k}},\frac{\log(n)}{n/k}\right\} \:,\]
and apply a union bound we get that with 
\[ \prob\left(\exists
i\: S_i \geq \expect[S_i] + t \,|\, \sim\mathcal{E}]\right) \leq n^{-\Omega(1)}
\:,\] and now substituting the value of $\expect[S(i) \,|\, \mathcal{E}]$ from
before and being extremely liberal with the the contants for $n$ large enough we
have that \[ \prob\left(\exists
i\:S(i) \geq  \frac{qn}{k} +
30\left(\sqrt{\frac{n\log(k)}{k}q} + \log(k) +
\sqrt{\frac{n}{k}\log(n)}\cdot
\max\left\{q,\sqrt{\frac{q\log(n)}{n/k}},\frac{\log(n)}{n/k}\right\}\right)\right)
\leq n^{-\Omega(1)}\:.\]

To show the second equation note that for any pair of clusters $t_1,t_2$,
$\delta_{P_{t_1}\rightarrow P_{t_2}}$ is a sum of $(n/k)^2$ independent random
variables. Therefore by a Chernoff bound from the second part of Theorem
\ref{thm:chernoff} and a union bound we get that with probability $1 - n^{-\Omega(1)}$
\[ \min_{t_1,t_2} \frac{\delta_{P_{t_1}\rightarrow P_{t_2}}}{n/k} \geq
\frac{qn}{k} - 2\sqrt{q\log(n)}\:.\]
\end{proof}
\subsubsection{Proof of Lemma \ref{lemma:edelta}}\label{subsec:edelta}
\begin{proof}
Consider $\delta_{\max}^{out}(i)$ for some $i$, this is defined to be the maximum
of $k$ random variables $S_i$ with $S_{i} \sim \mbox{Bin}(n/k,q)$ (the binomial
distribution with parameters $n/k,q$) with variance $\frac{n}{k}\sigma^2$ where
$\sigma^2 = q(1-q)$.
Consider $\tilde{S_{i}} = S_{i} - \expect[S_i]$. Let $\gamma =
\sigma\sqrt{\frac{n\log(k)}{k}} + \log(k)$. From Corollary
\ref{corr:mychernoffgood} we get that \[ \prob\left(\tilde{S_{i}} \geq 4(t+1)\gamma\right) \leq
\frac{1}{k^{t+1}} \:,\] therefore by a union bound we get that the \[
\prob\left(\max_i \tilde{S_{i}} \geq 4(t+1)\gamma\right) \leq
\frac{1}{k^t}\:.\] Hence, we can bound the expectation by
\begin{eqnarray*}
\expect[\max_i \tilde{S_i}] &\leq& 4\gamma + \sum_{t=1}^{\infty}
4(t+1)\gamma \, \prob\left(\max_i \tilde{S_i} \geq
4t\gamma\right)
\\
&\leq& 4\gamma + \sum_{t=1}^{\infty}
4(t+1)\gamma\frac{1}{k^{t-1}} \\
&\leq& 4\gamma +
4\gamma\left(\sum_{t=1}^{\infty}
(t+1)\frac{1}{2^{t-1}}\right) \\
&\leq& 4\gamma + 24\gamma \\
&\leq& 28\left(\sigma\sqrt{\frac{n\log(k)}{k}} + \log(k)\right)\:.
\end{eqnarray*} 
It follows from the above that
\[\expect[\delta_{\max}^{out}(i)] \leq \frac{n}{k}q +
28\left(\sqrt{\frac{n\log(k)}{k}q} + \log(k)\right)\:.\]
\end{proof}

\subsubsection{Proof of Uniqueness of the solution}
\label{sec:uniqueness}
In this section we prove that $Y^*$ is the unique optimal
solution to the SDP considered in section \ref{sec:proof_main_theorem}. To
remind the reader $M^*$ was the candidate dual solution. For the rest of the
section we use the same notations we defined in Sction
\ref{sec:proof_main_theorem}. To show uniqueness we make use of complementary
slackness which implies that for any other optimal solution $\hat{Y}$ since with high probability $M^* = D^* - \sum_i x_i^* R_i - A(G) - Z^*$ is an optimal solution of the dual program we have that
\begin{equation*} \hat{Y} \bullet M^* = 0 \:.\end{equation*}
But it is easy to see from the proof of Lemma \ref{lem:main_lemma} that we can
make a stronger statement that the subspace $\R_{k}$ is the
null space of $M^*$ and on the perpendicular subspace $\R_{n | k}$ the lowest eigenvalue is
strictly greater than 0. Combining this with the complementary slackness
condition in particular implies that the span of the columns of $\hat{Y}$ are
restricted to the span of $\R_{k}$. Hence, the conditions of
the SDP (sum constraint, the diagonal value constraint and the positivity constraint) force $\hat{Y} = Y^*$ if the column
space of $\hat{Y}$ is the span of $\R_{k}$ which proves
uniqueness.

\subsection{Analysis for SDP in \eqref{eqn:sdp2}}
\subsubsection{Proof of Theorem \ref{thm:main_theorem_sdp2}}
\label{sec:proofSDP2}
We extend the definitions of section \ref{sec:preliminaries} to ease
readability.
We define the notion of relative degree $\bar{\delta}$ by defining it as the
number of edges present minus the number of edges not present. In this light we define
the following quantities extending the definitions from Section
\ref{sec:preliminaries}

$\delta_{i \rightarrow P_t}$ to be the ``degree'' of vertex
$i$ to cluster $t$. Formally
\begin{eqnarray*} 
\bar{\delta}_{i \rightarrow P_t} &\defeq&  2\delta_{i \rightarrow P_t} - |P_t|
\\
\bar{\delta}_{P_{t_1} \rightarrow P_{t_2}}&\defeq& 2\delta_{P_{t_1} \rightarrow
P_{t_2}} - |P_{t_1}||P_{t_2}| \\
\bar{\delta}^{in}(i) &\defeq& 2\delta^{in}(i) - |P(i)| \\
\end{eqnarray*} 

We consider the following SDP in this section. Let $J$ be the $n \times n$
matrix such that $J[i,j] = 1$ for all $i,j$. 

\begin{equation} \begin{tabular}{l p{4cm} l}
    $\max$ & ${\displaystyle (2*A(G) - J)\bullet Y }$ & \\ 
    s.t.  & ${\displaystyle Y_{ii} = 1\;\; (\forall\;i)}$ \\
    & ${\displaystyle Y_{ij} \geq -\frac{1}{k-1}\;\; (\forall\;i,j)}$ \\
    & ${\displaystyle Y \succcurlyeq 0 }$ \:.
\end{tabular} \end{equation}

The dual of the above SDP is as follows

\begin{equation}\label{eqn:dual2} \begin{tabular}{l p{4cm} l}
    min & ${\displaystyle \mbox{Trace}(D) + \frac{1}{k-1}\sum_{ij} Z[i,j] }$ &
    \\
    s.t. & ${\displaystyle D - Z - (2A(G) - J)\succcurlyeq 0 \:. }$
\end{tabular} \end{equation} 

where $Z$ is a symmetric entrywise non-negative matrix with zeros in the
diagonal and $D$ is a diagonal matrix. 

The optimal solution $Y^*$ we have in mind is the matrix $Y^*_{ij} = 1$ if $i,j$
belong to the same cluster and $-\frac{1}{k-1}$ if $i,j$ belong to different
clusters. Note that $Y^*$ is PSD and is a valid solution of the primal. In
this case it is easy to see that the value of the SDP is equal to \[ (2*A(G) - J)\bullet Y^* = \sum_i
\left(\bar{\delta}_{in}(i) - \frac{\sum_{t:P(i) \neq P_t} \bar{\delta}_{i
\rightarrow P_t}}{k-1} \right)\]
We will exhibit a candidate dual solution $D^*,Z^*$ such that 
\[ (2*A(G) - J)\bullet Y^* = \mbox{Trace}(D) + \frac{1}{k-1}\sum_{ij} Z[i,j]\]
and with high probabiltiy $D^* - Z^* - (2A(G) - J)\succcurlyeq 0$ if condition
\eqref{eqn:sdp2_condition} of the theorem is satisfied. Note that this implies
through weak duality that $Y^*$ is a solution of \eqref{eqn:sdp2}. The
Uniqueness of the solution can be proved exactly in the same way as in Section
\ref{sec:uniqueness}

Before we define our candidate dual solution we define the following quantity
for ease of notation. 
\begin{equation}
\label{eqn:defmin}
\bar{\delta}_{min} \defeq \min_{i,j} \left( -\bar{\delta}_{i \rightarrow
P(j)} - \bar{\delta}_{j \rightarrow P(i)}  + \frac{\bar{\delta}_{P(j)
\rightarrow P(i)}}{(n/k)} \right) = \left( n/k - 2 \max_{i,j} \left(\delta_{i
\rightarrow P(j)} + \delta_{j \rightarrow P(i)} - \frac{\delta_{P(j)
\rightarrow P(i)}}{(n/k)}  \right) \right)
\end{equation}

We begin by describing the choice of $Z^*$. If vertex $i$ and $j$ belong to the
same clusters then $Z^*[i,j] = 0$ otherwise
\begin{equation*}
    Z^*[i,j] \defeq \left( -\frac{\bar{\delta}_{i \rightarrow P(j)}}{n/k}
    -\frac{\bar{\delta}_{j \rightarrow P(i)}}{n/k} 
    + \frac{\bar{\delta}_{P(j) \rightarrow P(i)}}{(n/k)(n/k)} - 
    \frac{\bar{\delta}_{min}}{n/k} \right) = \left( 1 - 2\left(\frac{\delta_{i
    \rightarrow P(j)}}{n/k} + \frac{\delta_{j \rightarrow P(i)}}{n/k} 
    - \frac{\delta_{P(j) \rightarrow P(i)}}{(n/k)(n/k)}\right) - 
    \frac{\bar{\delta}_{min}}{n/k} \right)
\end{equation*}

Note that by definition (\ref{eqn:defmin}) $Z^*$ is a symmetric non-negative
matrix.
We now define the diagonal matrix $D^*$ as 
\begin{equation*}
D^*[i,i] \defeq \bar{\delta_{in}(i)} + \bar{\delta}_{min} = 2\left(
\delta_{in}(i) - \max_{i,j} \left(\delta_{i
\rightarrow P(j)} + \delta_{j \rightarrow P(i)} - \frac{\delta_{P(j)
\rightarrow P(i)}}{(n/k)} \right)\right)
\end{equation*}

A simple calculation now shows the first required property that 
\[ \mbox{Trace}(D) + \frac{1}{k-1}\sum_{ij} Z[i,j] = \sum_i
\left(\bar{\delta}_{in}(i) - \frac{\sum_{t:P(i) \neq P_t} \bar{\delta}_{i
\rightarrow P_t}}{k-1}\right) = (2*A(G) - J)\bullet Y^*\]

We now proceed to show that $D^*,Z^*$ is a valid dual solution, i.e.
\[ M^* = D^* - Z^* - (2A - J) \succeq 0\] To see
this consider the following extension of the decomposition of the space $\R^n$
defined in section \ref{sec:proof_main_theorem}.

\begin{definition}
\label{def:spaces2}
Given a $k$-clustering of $n$ vertices $\{P_t\}_{t=1}^k$ we define the vectors
$v_t$ to be the indicator vectors of the clusters. We further define the
following subspaces, which are perpendicular to each other, and partition $\R^n$.
\begin{itemize}
\item $\allone$: the vectors with 1 in each coordinate
\item $\R_{k-1}$: the $k-1$ dimensional subspace such that for every vector $v
\in \R_{k-1}$, $v(i)=v(j)$ if $P(i)=P(j)$ and $<v,\allone> = 0$
\item $\R_{n | k}$: the subspace perpendicular to $\R_{k-1} \cup \allone$, i.e.
the subspace where the sum on each cluster is equal to 0.
\end{itemize}
\end{definition}

Following are two easy observations that follow from simple calculations
similar to the calculations shown in Section \ref{sec:proof_main_theorem}. 
\begin{observation}
$(\forall\;\;v \in \R_{k-1})\; (D^* - Z^* - (2A - J))v = 0$
\end{observation}
\begin{observation}
$(\forall\;\;v \in \R_{n | k})\; v^TZ^*v = 0$
\end{observation}

We first focus on the subspace $\R_{n | k}$ and show that $\forall x \in \R_{n
| k}$
\begin{equation}
 x^T(D^* - Z^* - (2A - J)x = x^T(D^* - 2A)x \geq 0
\end{equation}
The proof of the above statement follows from the following set of inequalities
\begin{eqnarray*}
x^T(D^* - 2A)x \geq &\min_i& D^*[i,i] - 2\max_{x} x^TA(G)x \\
&\geq& 2\min_i \nu(i) - 2\max_{x} x^TA(G)x \\
&\geq& 2\left(\min_i \nu(i) - \hat{c}\left(\sqrt{pn/k + qn} +
 + \sqrt{\log(n)}\right) \right) \\
 &\geq& 0
\end{eqnarray*}
where the second inequality above follows from substituting the values of
$\bar{\delta}_{i \rightarrow P(t)}$ in terms of $\delta_{i \rightarrow P(t)}$ in
the expression for $D^*[i,i]$ and using the definition of $\nu (i)$. The second
inequality follows from Lemma \ref{lemma:conc} and third inequality follows
from the condition \eqref{eqn:sdp2_condition}. Note that in condition
\eqref{eqn:sdp2_condition} if we assume the constant to be $\hat{c} + 1$ instead
of $\hat{c}$ then we get a stronger property that the above quantity is in fact
greater than $\sqrt{\log(n)}$ and not just positive. We use this below. 

The above analysis shows that the matrix $M^* = D^* - Z^* - (2A - J)$ is PSD on
the subspace $\R_{n | k}$. Lets now focus on a vector $y \in \R_{n | k} \oplus
\allone$. Let $H^* = D^* - Z^* - 2A = M^* - J$. By appropriate scaling we can
consider any $y = x  + \delta \frac{\allone}{\sqrt{n}}$ (see footnote
\footnote{Indeed by definition any vector $y \in \R_{n | k} \oplus
\allone$ can be written as $x +
\delta \frac{\allone}{\sqrt{n}}$ for some $\delta$ and $x \in \R_{n | k}$. For
the purpose of proving positive definiteness we can always divide by any positive
number and can there fore consider $\frac{y}{\|x\|}$. Also note that we can
consider $y$ or $-y$ equivalently and hence can consider the case when $\delta > 0$.}) where $x \in
\R_{n | k}$ is a unit vector and $\delta \geq 0$. In the analysis above we explained that 
$x^TH^*x \geq \sqrt{\log(n)}\|x\|^2 = \sqrt{\log(n)}$.
With these facts in place consider $y^TM^*y$
\begin{eqnarray*}
y^TM^*y &=& x^TH^*x + \frac{\delta^2}{n}\allone^T J \allone +
2x^TH^*\frac{\delta}{\sqrt{n}}\allone \\
&\geq& \sqrt{\log(n)} + \delta^2 n - 2\delta\|H^*\| 
\end{eqnarray*} 

where we use the fact that for unit vector $x$ $\frac{x^TH^*\allone}{\sqrt{n}}
\leq \|H^*\|$. Therefore as long as we have that $4\|H^*\|^2 \leq
4n\sqrt{\log(n)}$ we have that that $y^TM^*y \geq 0$ (as the expression is a quadratic in
$\delta$). Therefore we need to control the spectral norm of $H^*$. We can show
the above via very simple and fairly loose calculations

\begin{eqnarray*}
\|H^*\| &\leq& \|D^*\| + 2\|A\| + \|Z^*\| \\
&\leq& \max D^*[i,i] + 2\delta_{max} + O(\delta_{max}) \\
&\leq& O(\delta_{max})
\end{eqnarray*}

where $\delta_{max}$ is the degree of the vertex with maximum degree in the
graph $G$. The above equation follows with very loose aproximations from the
definitions. A simple chernoff bound shows that with high probability
$\delta_{max} \leq pm + kqm + \sqrt{pm + kqm}\log(n) \leq O(k\log(n) +
\log^{3/2}(n))$ where we have replaced $p$  with $\alpha\frac{\log(m)}{m}$ and
$q$ with $\beta\frac{\log(m)}{m}$ which implies that $\|H^*\| \leq \sqrt{n}$
which completes the proof since we have shown that $M^*$ is PSD.

\subsection{Monotone Adversary - Proof of Theorem \ref{thm:adversary}}
\label{sec:adversaryproof}
\begin{proof}
We consider the SDP relaxation (\ref{eqn:sdp}) as in the proof of Theorem
\ref{thm:main_theorem_1_opt}.
Let $Y^*(G)$ be the optimal solution of the SDP when we run it on the graph
$G$.
Now suppose $G \sim \mathcal{G}_{p,q,k}$. The proof of Theorem
\ref{thm:main_theorem_1_opt} shows that with high probability, $Y^*(G)$
is unique and it corresponds to the hidden partition. Suppose this event happens, we then show that for any graph
$G_{adv}$ generated by the monotone adversary after acting on $G$, $Y^*(G_{adv})$ is also unique and it is equal to $Y^*(G)$. This will prove
Theorem \ref{thm:adversary}.

Define $SDP_{G}(Y)$ to be the objective value (corresponding to the graph $G$)
of a feasible matrix $Y$, i.e. $SDP_{G}(Y) = A(G)\bullet Y$. Note that since $Y$
has only positive entries (since it is a feasible solution) we have that
$A(G')\bullet Y \leq A(G) \bullet Y$, if $G'$ is a subgraph of $G$. Also since
$Y \succeq 0$ and its diagonal entries $Y_{ii} = 1$ we have that $|Y_{ij}| \leq
1$. Therefore $A(G\cup{e})\bullet Y \leq A(G) \bullet Y + 2$.
Suppose the monotone adversary adds a total of $r^+$ edges and removes $r^-$
edges. From the monotonicity of the adversary it is easy to see that
$A(G_{adv})\bullet Y^*(G) = A(G)\bullet Y^*(G) + 2r^+$. However for any other
solution by the argument above we have that $A(G_{adv})\bullet Y \leq
A(G)\bullet Y + 2r^+$. Also by our assumption we have that $A(G) \bullet Y^*(G)
< A(G) \bullet Y$ for any feasible $Y \neq Y^*(G)$. Putting it together we have
that 
\[ A(G_{adv})\bullet Y^*(G) = A(G)\bullet Y^*(G) + 2r^+ > A(G)\bullet Y + 2r^+
\geq A(G_{adv})\bullet Y \:,\]
for any feasible $Y \neq Y^*(G)$, which proves the theorem.
\end{proof}

\subsection{Forms of Chernoff Bounds and Hoeffding Bounds Used in the Arguments}
\begin{theorem}[Chernoff]
\label{thm:chernoff}
Suppose $X_1 \ldots X_n$ be independent random variables taking values in
$\{0,1\}$. Let X denote their sum and let $\mu = \expect[X]$ be its expectation. Then for any $\delta > 0$ it holds that
\begin{equation}
\prob\left( X > (1 + \delta)\mu\right) < \left(\frac{e^{\delta}}{(1 +
\delta)^{(1+\delta)}}\right)^{\mu}\:,
\end{equation}
\begin{equation}
\prob\left( X < (1 - \delta)\mu\right) < \left(\frac{e^{-\delta}}{(1 -
\delta)^{(1-\delta)}}\right)^{\mu} \:.
\end{equation}
A simplified form of the above bound is the following formula (for $\delta \leq
1$) \[\prob\left( X \geq (1 + \delta)\mu\right) \leq e^{-\frac{\delta^2 \mu}{3}}\:, \]
\[\prob\left( X \leq (1 - \delta)\mu\right) \leq e^{-\frac{\delta^2 \mu}{2}}
\:.\]

\end{theorem}

%I realized later that I can also derive the above statement using Bernstein's
%inequality
\begin{theorem}[Bernstein]
\label{thm:normalBernstein}
Suppose $X_1 \ldots X_n$ be independent random variables taking values in
$[-M,M]$. Let X denote their sum and let $\mu = \expect[X]$ be its expectation, then
\[ \prob\left( |X - \mu| \geq t \right) \leq
\exp\left(-\frac{1}{2}\frac{t^2}{\sum_i \expect[(X_i - \expect[X_i])^2] + Mt/3}\right) \:. \]
\end{theorem}

\begin{corollary}
\label{corr:mychernoffgood}
Suppose $X_1 \ldots X_n$ are i.i.d Bernoulli variables with parameter $p$. Let
$\sigma = \sigma(X_i) = p(1-p)$ then we have that for any $r\geq 0$
\[\prob\left(X \geq
\mu + \alpha\sigma\sqrt{n\log(r)}+ \alpha\log(r)\right) \leq e^{-\frac{\alpha\log(r)}{4}} \:.\]
\end{corollary}
\begin{proof}
We have that $n\sigma^2 = np(1-p)$ and $M = 1$. We can now choose $t =
\alpha\sigma\sqrt{n\log(r)} + \alpha\log(r)$. This implies that $\frac{n\sigma^2
+ t/3}{t^2} \leq \frac{1}{\log(r)}\left(1/\alpha^2 + 1/3\alpha\right) \leq
\frac{2}{\alpha\log(r)} $ which implies from Theorem \ref{thm:normalBernstein}
that $\prob\left(X > \mu + \alpha\sigma\sqrt{n\log(r)}+ \alpha\log(r)\right) \leq e^{-\frac{\alpha\log(r)}{4}}.$
\end{proof}

\begin{theorem}[Hoeffding]
\label{thm:Hoeffding}
Let $X_1 \ldots X_n$ be independent random variables. Assume that the $X_i$ are
bounded in the interval $[a_i,b_i]$. Define the empirical mean of these
variables as
\[ \bar{X} = \frac{\sum_i \bar{X_i}}{n} \:, \]
then 
\begin{equation}
\prob\left( |\bar{X} - \expect[\bar{X}]| \geq t \right) \leq 2\exp\left(-
\frac{2n^2t^2}{\sum_{i = 1}^{n} (b_i - a_i)^2}\right) \:.
\end{equation}
\end{theorem}
